# Supplementary material for: Improved Bounds for Private and Robust Alignment
Source: arXiv:2512.23816 source file (2026-06-25)
Supplement: Supplementary file 1 [file app-comparison.tex]

\section{Summary Comparison with Prior Work}
\label{app:comparison}

% To facilitate comparison with existing results, we summarize the main theoretical guarantees across different alignment settings in Tables~\ref{tab:offline-comparison} and~\ref{tab:online-comparison}.
% The table highlights the loss function, privacy and corruption assumptions, and the resulting convergence guarantees in both offline and online regimes.

To facilitate comparison with existing results, we summarize the main theoretical guarantees across different alignment settings in Tables~\ref{tab:offline-comparison} and~\ref{tab:online-comparison}.
These tables highlight the loss function, privacy and corruption assumptions, and the resulting convergence guarantees in both offline and online regimes.

Our improvements over prior work are primarily reflected in two aspects: 
(i)~we achieve polynomial improvements in corruption dependence from $\sqrt{\alpha}$ to $\alpha$ in the offline setting, and (ii)~we are the first to provide optimal rates for MLE-type log loss under differential privacy constraints.

\begin{table}[H]
    \centering
    \caption{Summary of theoretical guarantees in the \emph{offline} alignment setting. Here $\kappa(\pi^\star)$ denotes the single-policy concentrability coefficient.}
    \label{tab:offline-comparison}
    \small
    \begin{tabular}{lccc}
        \toprule
        Method & Loss & Scenario & Theoretical Bound \\ 
        \midrule
        Square$\chi$PO~\cite{zhou2025square} 
        & Square 
        & Private + Corruption 
        & $\begin{aligned}
                \textsf{CTL: } & O\!\left(\kappa(\pi^\star)\!\left(c(\epsilon)\sqrt{\tfrac{\log(|\Pi|/\delta)}{n}} + \sqrt{\alpha}\right)\right)\\
                \textsf{LTC: } & O\!\left(\kappa(\pi^\star)\!\left(c(\epsilon)\sqrt{\tfrac{\log(|\Pi|/\delta)}{n}} + \sqrt{c(\epsilon)\alpha}\right)\right)
            \end{aligned}$ \\

        Square$\chi$PO (Ours) 
        & Square 
        & Private + Corruption 
        & 
        $\begin{aligned}
            \textsf{CTL: } & O\!\left(\kappa(\pi^\star)\!\left(c(\epsilon)\sqrt{\tfrac{\log(|\Pi|/\delta)}{n}} + \alpha\right)\right)\\
            \textsf{LTC: } & O\!\left(\kappa(\pi^\star)\!\left(c(\epsilon)\sqrt{\tfrac{\log(|\Pi|/\delta)}{n}} + c(\epsilon)\alpha\right)\right)
        \end{aligned}$ \\

Priv$\chi$PO (Ours) 
& Log (MLE) 
& Private only 
& 
$O\!\left(\kappa(\pi^\star)\,c(\epsilon)\sqrt{\tfrac{\log(|\Pi|/\delta)}{n}}\right)$ \\

\bottomrule
\end{tabular}
\end{table}

\begin{table}[H]
\centering
\caption{Summary of theoretical guarantees in the \emph{online} alignment setting.
Here $\kappa_{\mathrm{cov}}(\Pi)$ denotes the coverability coefficient.}
\label{tab:online-comparison}
\small
\begin{tabular}{lccc}
\toprule
Method & Loss & Scenario & Theoretical Bound \\ 
\midrule
XPO~\cite{xie2024exploratory} 
& Log (MLE) 
& Non-private 
& 
$O\!\left(\kappa_{\mathrm{cov}}(\Pi)\sqrt{\tfrac{\log(|\Pi|T)}{T}}\right)$ \\

SquareXPO (Ours) 
& Square 
& Private + Corruption 
& 
$\begin{aligned}
\textsf{CTL: } & O\!\left(\kappa_{\mathrm{cov}}(\Pi)\!\left(c(\epsilon)\sqrt{\tfrac{\log(|\Pi|T/\delta)}{T}} + \alpha\right)\right)\\
\textsf{LTC: } & O\!\left(\kappa_{\mathrm{cov}}(\Pi)\!\left(c(\epsilon)\sqrt{\tfrac{\log(|\Pi|T/\delta)}{T}} + c(\epsilon)\alpha\right)\right)
\end{aligned}$ \\[1.2em]

PrivXPO (Ours) 
& Log (MLE) 
& Private only 
& 
$O\!\left(\kappa_{\mathrm{cov}}(\Pi)\,c(\epsilon)\sqrt{\tfrac{\log(|\Pi|T/\delta)}{T}}\right)$ \\

\bottomrule
\end{tabular}
\end{table}
